# Supplementary material for: Faceting transition in aluminum as a grain boundary phase transition
Source: arXiv:2506.13550 ancillary file (2025-09-24)
Supplement: Supplementary file 1 [file supplemental-material.pdf]

# SUPPLEMENTAL MATERIAL

# Faceting transition in aluminum as a grain boundary phase transition

Yoonji Choi (최윤지) and Tobias Brink

*Max Planck Institute for Sustainable Materials, Max-Planck-Straße 1, 40237 Düsseldorf, Germany*

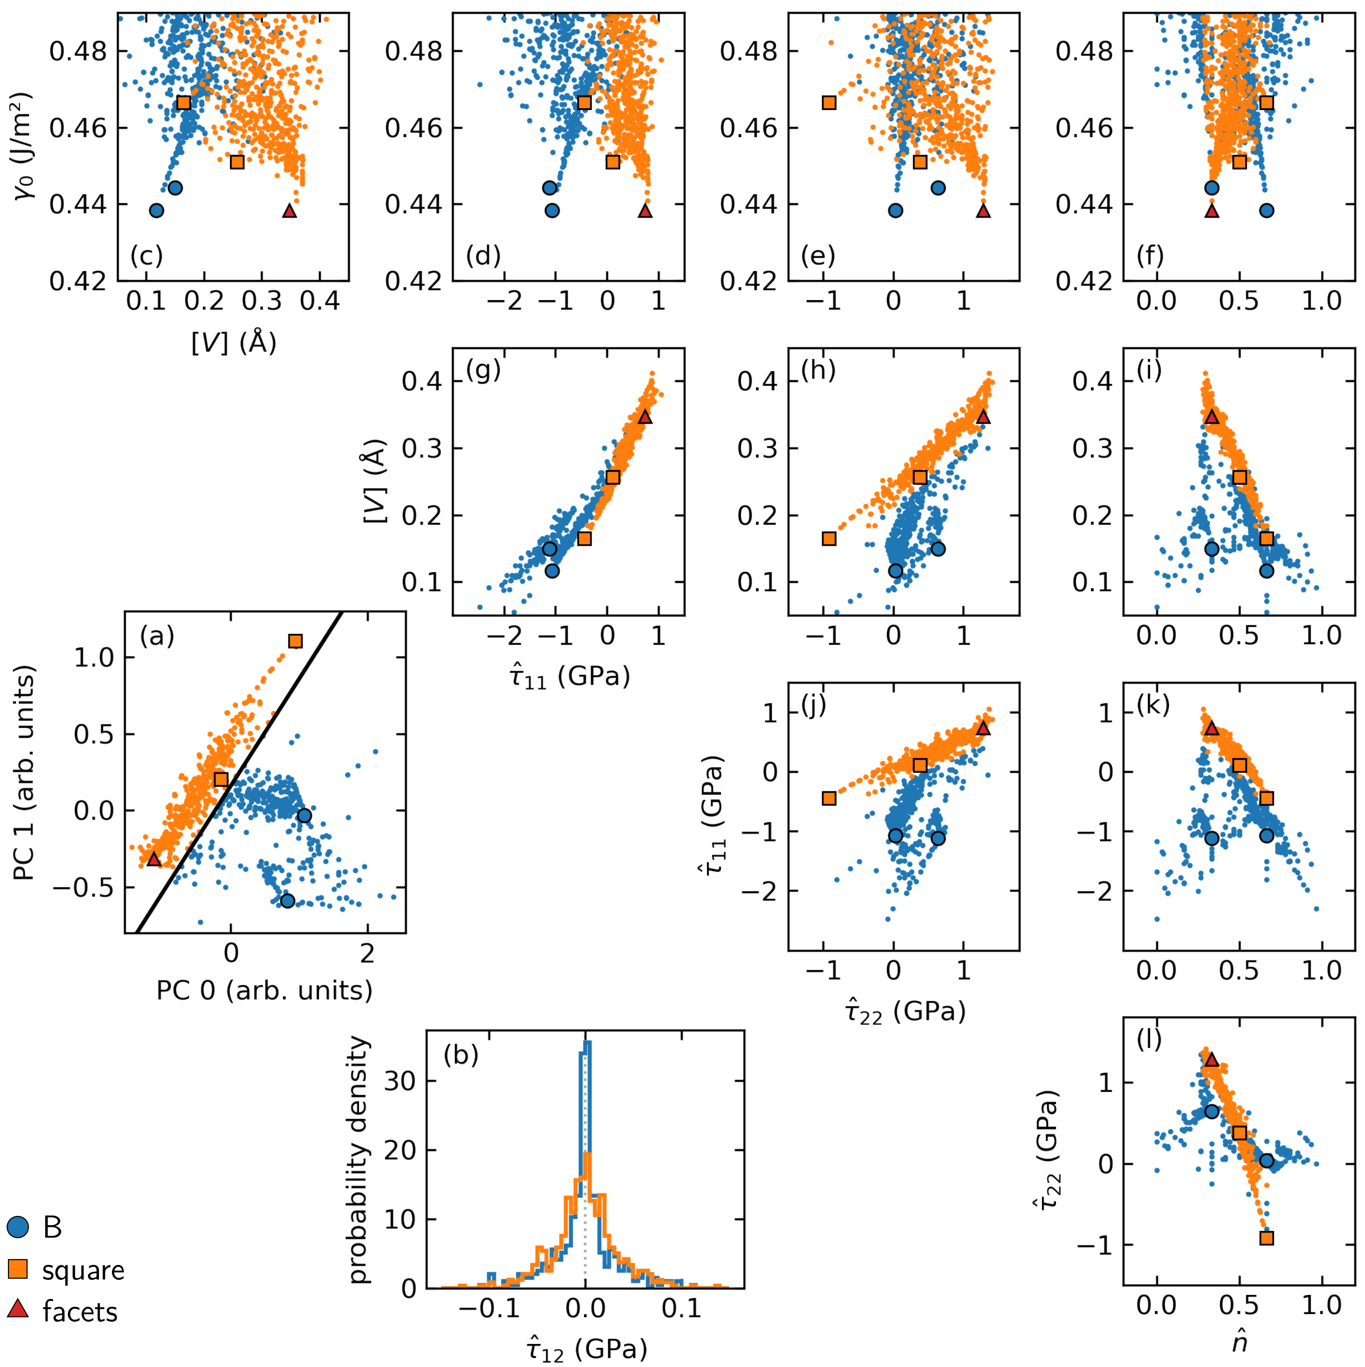


**Supplemental Fig. S1:** Results of the structure search for Σ3 [11$\bar{1}$] (011) GBs using GRIP with the Zha09 potential. Here, the excess properties of all found structures are plotted (each data point is a structure), with the lowest-energy representatives of the B, square, and faceted zipper phases marked with larger symbols. (a) First, we performed a principal component analysis to separate the data points into clusters. We used $\gamma_0$, $[V]$, $\hat{\tau}_{11}$ and $\hat{\tau}_{22}$ as descriptors for this. We excluded $\hat{\tau}_{12}$ because all structures seem to be distributed equally around $\hat{\tau}_{12} = 0$ (b). Additionally, $\hat{n}$ is not a useful descriptor, since defects or variations in the same GB phase can have different $\hat{n}$ values, such as e.g. B ⅓ and B ⅔. We separated the data by the line drawn in panel (a), coloring all data points according to this separation in either blue or orange. (c)–(l) Pair plots of all combinations of excess properties.

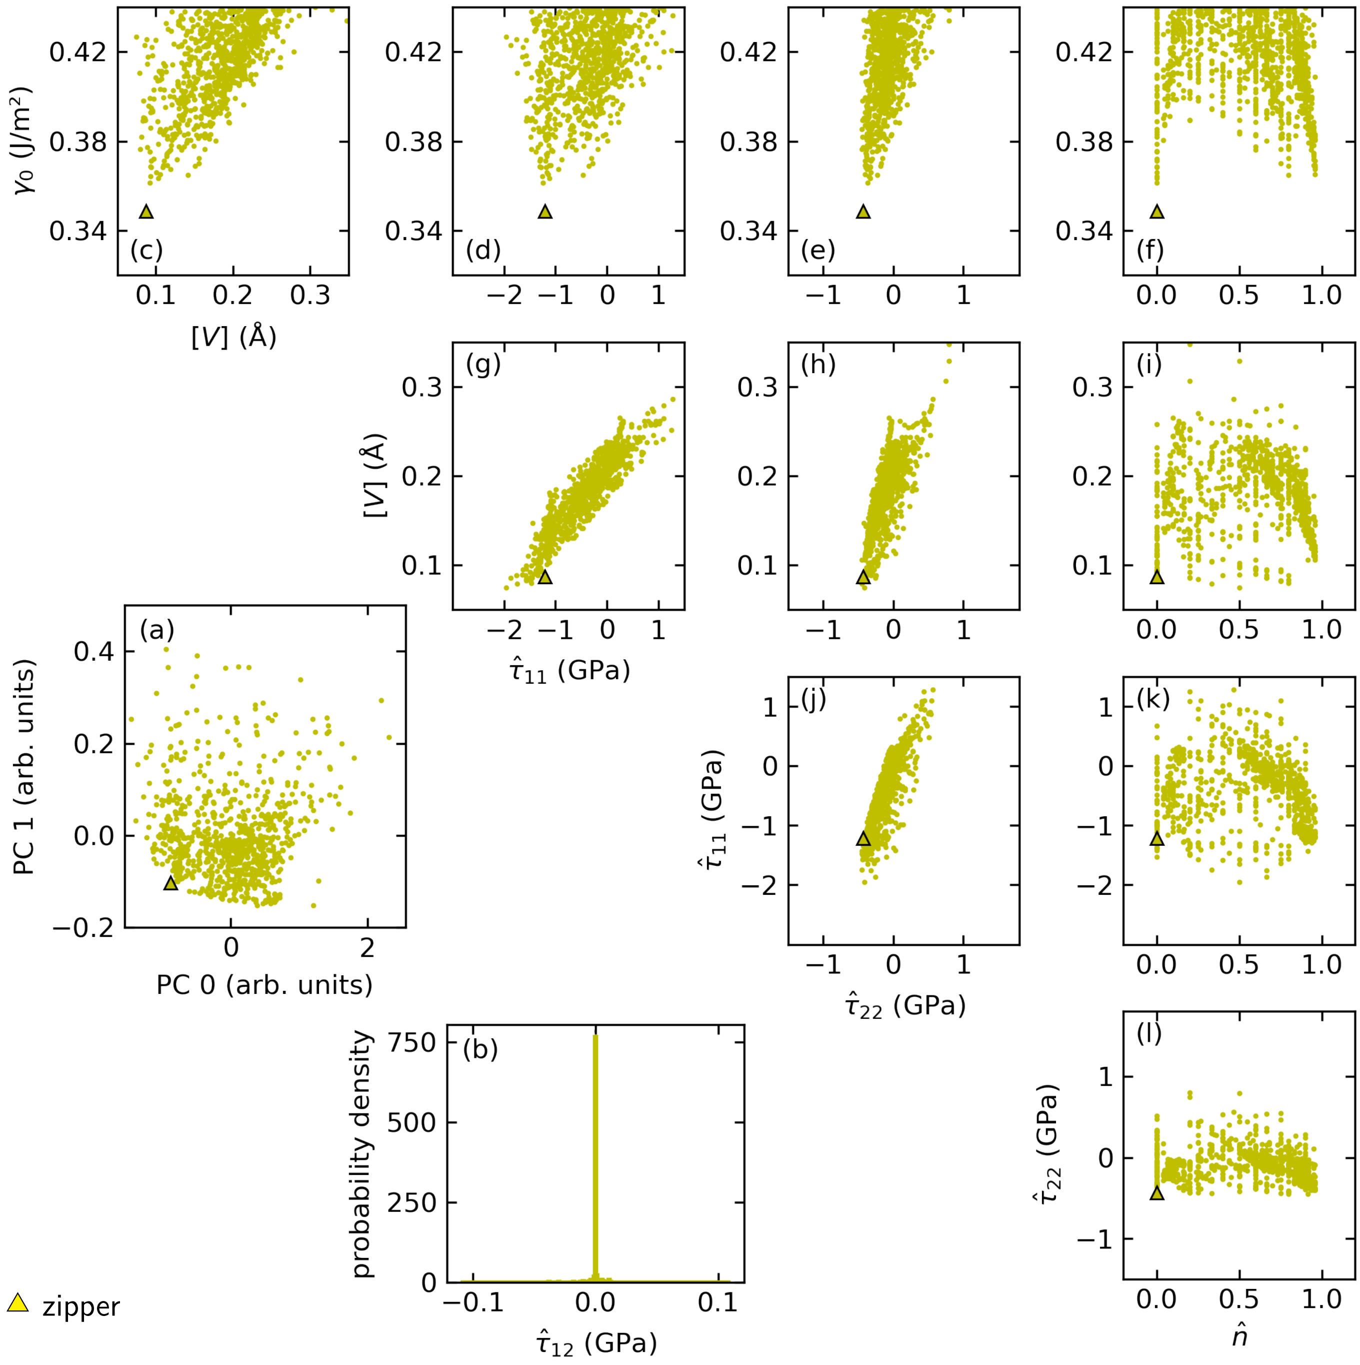


**Supplemental Fig. S2:** Results of the structure search for $\Sigma 3$ $[11\bar{1}]$ (112) GBs using GRIP with the Zha09 potential. Here, the excess properties of all found structures are plotted (each data point is a structure), with the perfect zipper structure marked with a larger symbol. (a) We performed a principal component analysis in the same way as in Supplemental Fig. S1(a). Only a single cluster can be found. (b) The value of $\hat{\tau}_{12}$ is approximately zero for all structures due to the symmetry of the GB. (c)–(l) Pair plots of all combinations of excess properties.

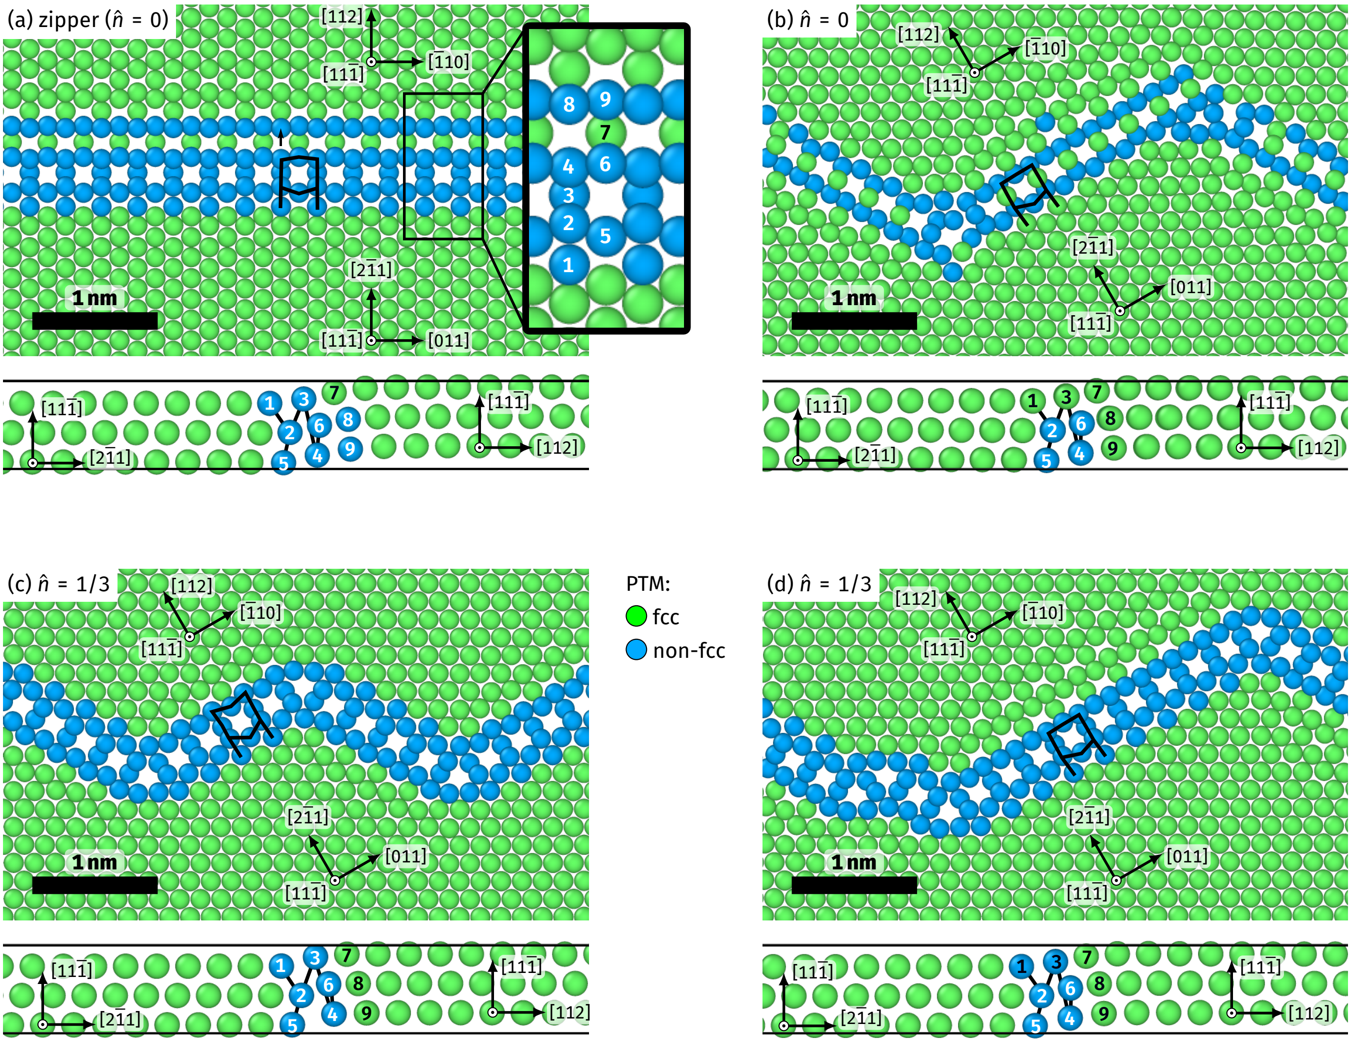


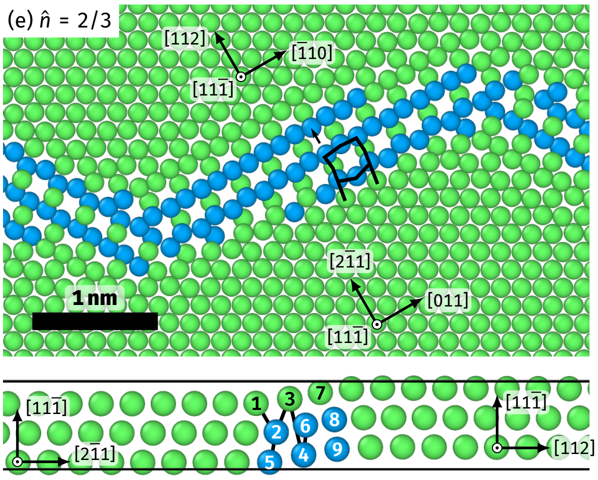


**Supplemental Fig. S3:** Comparison of the atomic structure of various zipper GBs obtained from GRIP or by construction. The color coding corresponds to the results of the polyhedral template matching (PTM) algorithm, with green atoms being fcc and all non-fcc atoms being colored in blue. (a) We arbitrarily mark a structural unit in the perfect zipper structure (black lines in the rough shape of an "A"). For later reference, we number the atoms in the motif's unit cell as indicated in the inset. Additionally to the marked motif, there is a line of atoms above this motif that are also identified as non-fcc. The small arrow indicates the displacement of atom 8 from the ideal fcc position. In the bottom, a cross-sectional view is shown. (b)–(e) For the faceted structures, PTM results are not matching to the ideal zipper structure. However, this analysis is affected by strains due to the facet junctions. In all cases, we can find the marked motif again in the GB. The cross-sectional views also reveal that the zipper structures are all the same except for some elastic distortion.

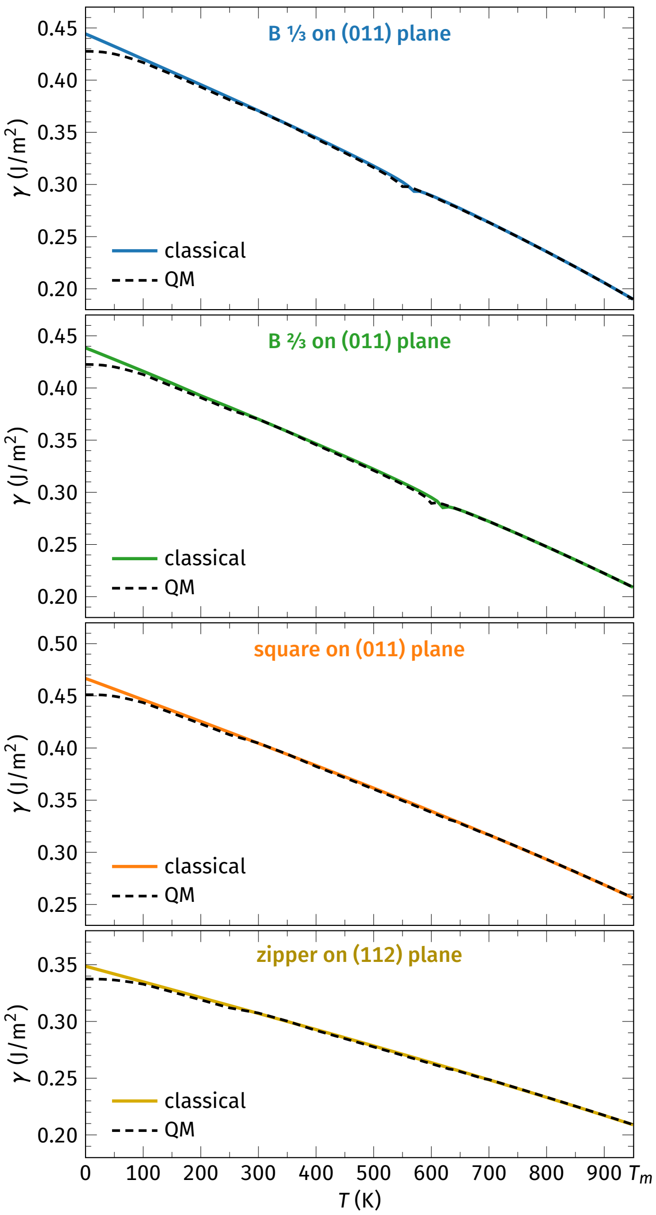


**Supplemental Fig. S4:** Excess free energies of the GB phases as a function of temperature, computed with the Zha09 potential. Here, we compare the calculations using the assumption of a classical system (solid, colored lines) to excess free energies including quantum-mechanical effects (QM, dashed lines). For the classical systems, thermal expansion was determined using MD simulations on an fcc crystal in which the system was equilibrated for 1 ns at each temperature, using 50 K temperature steps. Then the free energy was calculated using Eq. 8 in the main paper. For the quantum-mechanical calculation, we instead computed the free energy of fcc Al using Eq. 9 in the main paper for a range of volumes. At each temperature, the volume with the lowest free energy was chosen as the equilibrium volume. In all cases, the plotted excess free energy is the one defined by Eq. 4 in the main paper, i.e., $\gamma = [F]$, where $F$ was obtained at the equilibrium volume for each given temperature. The Debye temperature of Al is 428 K (C. Kittel, *Introduction to Solid State Physics*, Wiley, Hoboken, New Jersey, USA, 2005), but we can see from the data that the *excess* free energy is only different between classical and quantum mechanics up to around 100 K. This can be mostly attributed to zero-point vibrations. Other quantum effects cancel out in the excess calculation.

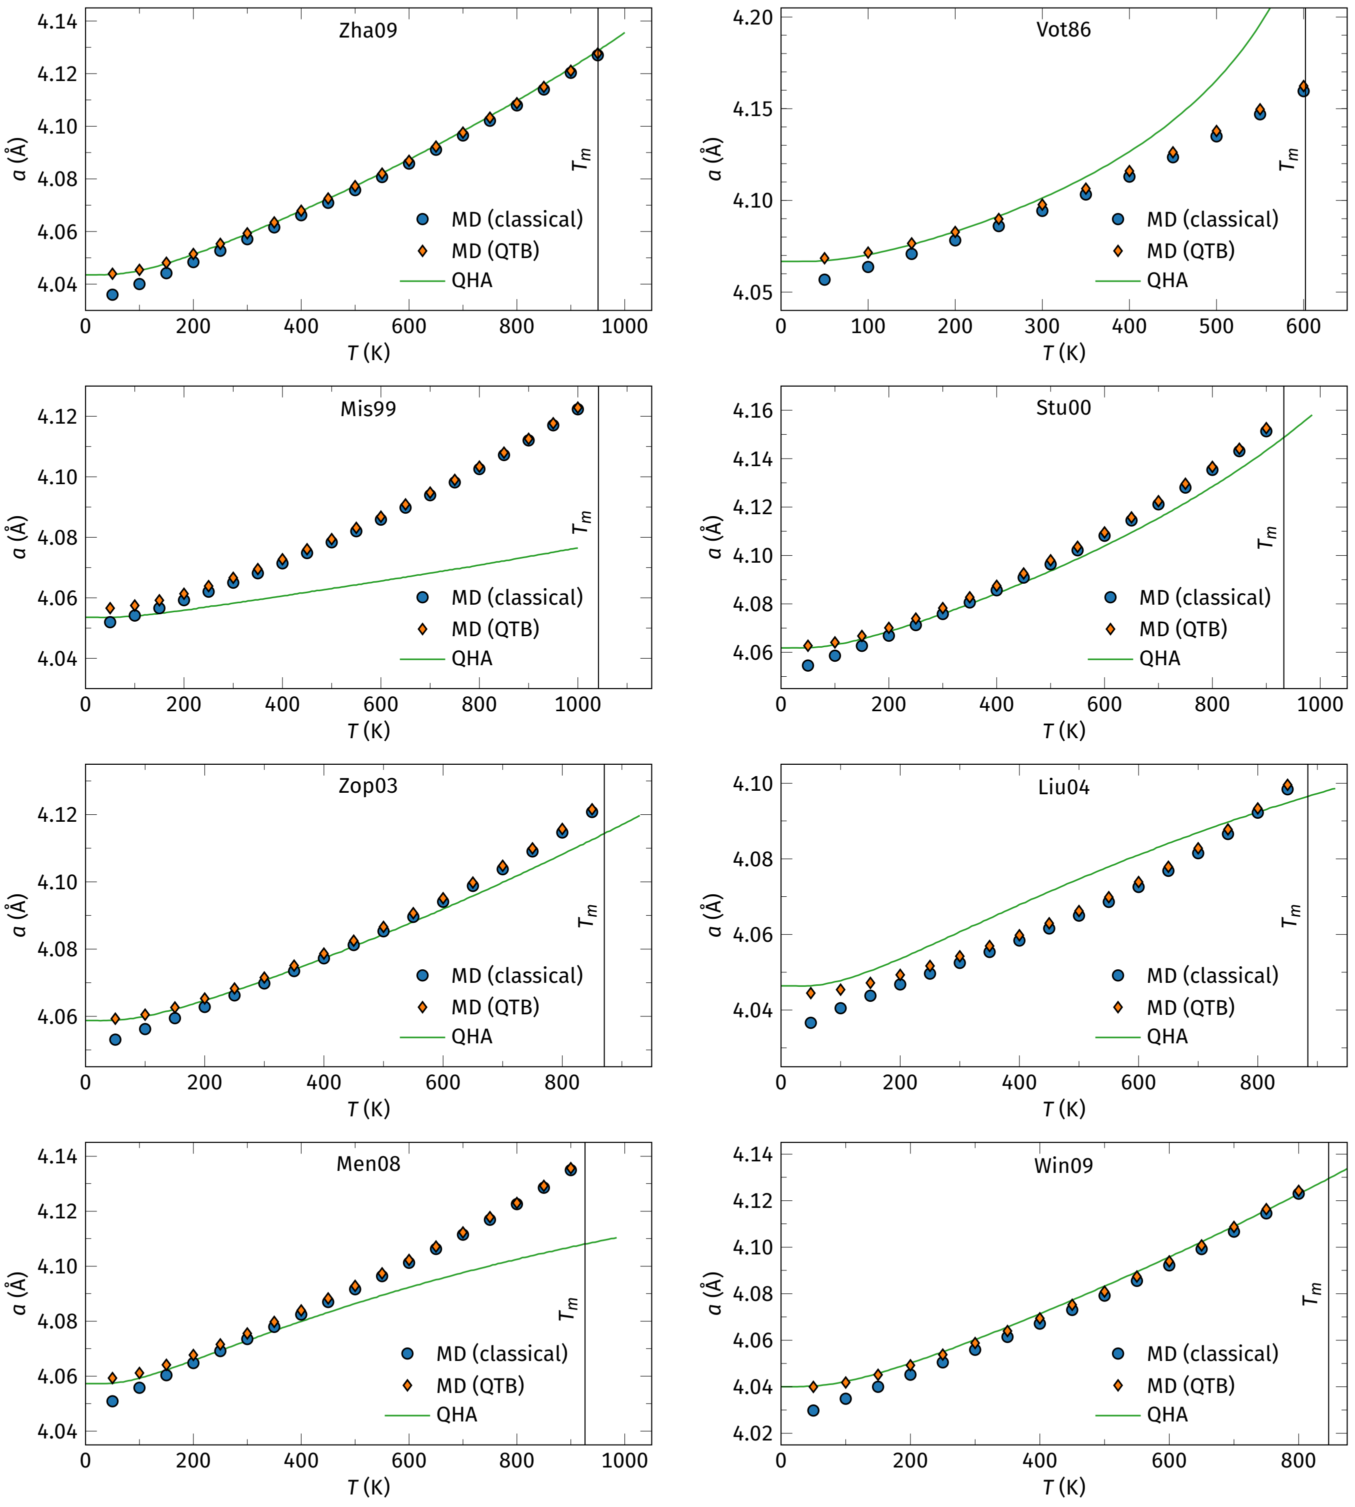


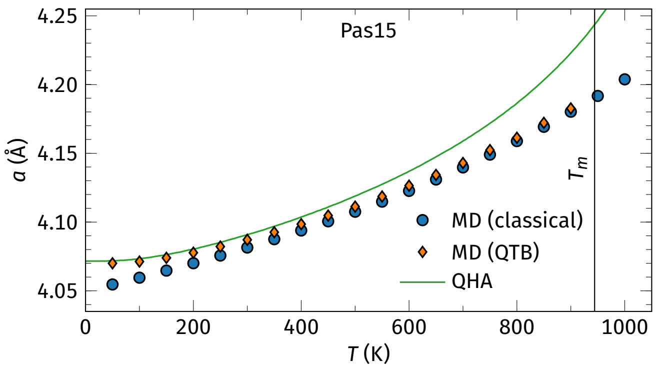


**Supplemental Fig. S5:** Lattice constants computed using different methods for different potentials. We calculated the lattice constants using classical mechanics with MD as also described in Supplemental Fig. S4. Additionally, we used a quantum thermal bath (QTB) to compute lattice constants including quantum-mechanical effects. Finally, we used the quasi-harmonic approxmination (QHA) as implemented in PHONOPY with finite displacements of 0.01 Å. Classical and quantum mechanical calculations agree at high temperatures, but many potentials lead to wrong predictions using the QHA.

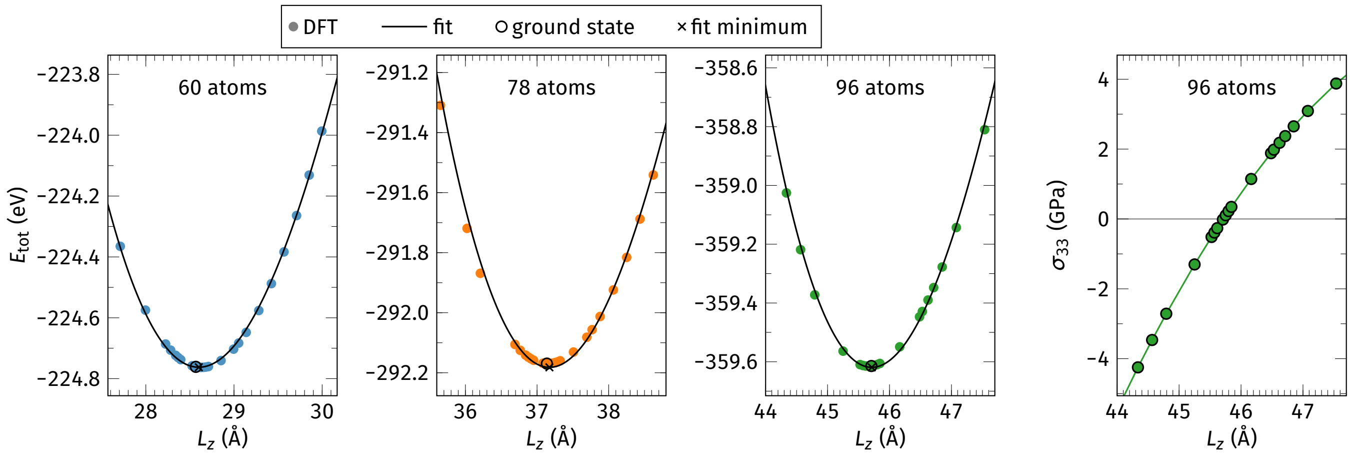


**Supplemental Fig. S6:** DFT calculations on an fcc cell with crystal direction $[11\bar{1}]$ in $x$, $[\bar{2}1\bar{1}]$ in $y$, and [011] in $z$. We used the minimal periodic size in $x$ and $y$ and varied the number of repeating cells in $z$ (different number of atoms). Then, we fixed the cell size according to the lattice constant computed with the same DFT parameters (4.040 Å). Finally, we performed calculations where the cell length $L_z$ was varied to produce reference data for GB excess calculations under stress $\sigma_{33}$. The stress (righmost plot) was calculated as $\sigma_{33} = (\mathrm{d}E_{\mathrm{tot}}/\mathrm{d}L_z)/(L_x L_y)$ by fitting a third order polynomial to the energy (black lines). We plot both the ground state for the unstretched cells (circles) and the minimum of the fit curve (crosses). These values coincide within the margin of error, as expected.

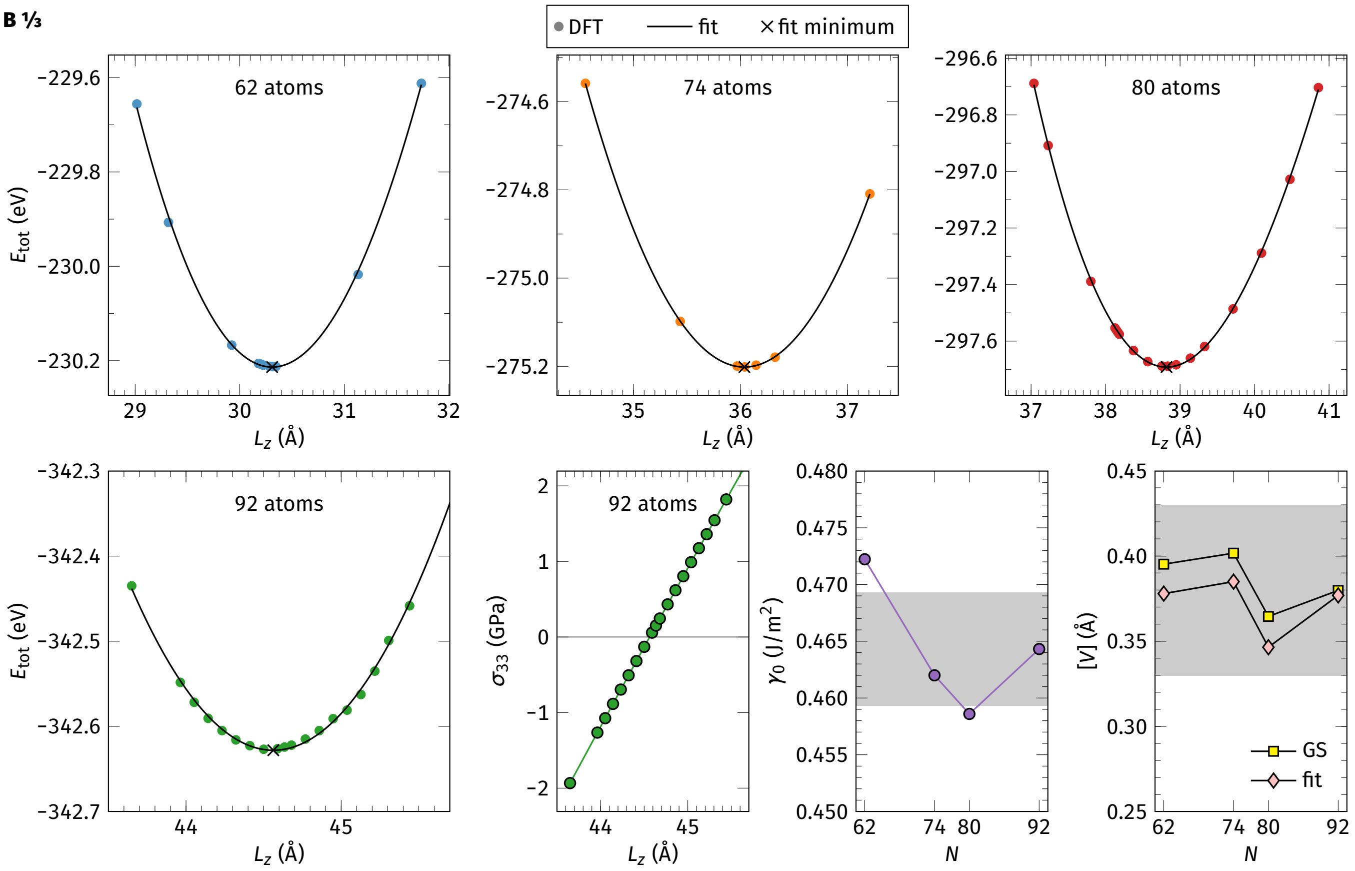


**Supplemental Fig. S7:** The same calculations as in Supplemental Fig. S6 were performed on cells additionally containing two equivalent GBs (here B ⅓). The number of atoms correlates with the cell size in $z$ direction and therefore with the amount of bulk material between the GBs. The excess values $\gamma_0$ and $[V]$ are converged with system size. The gray areas represent our conservative estimates of the errors $\Delta\gamma_0 = \pm 0.005\,\mathrm{J/m^2}$ and $\Delta[V] = \pm 0.05$ Å. We calculated the excess volume $[V]$ once with reference to the ground-state fcc cell (GS) and once with reference to the minimum of the polynomial for $E_{\mathrm{tot}}(L_z)$ (fit). Those values converge for the largest cell. Excess properties were calculated with reference to the fcc cell closest in size. An exact match in number of atoms is not possible for $\hat{n} \neq 0$, by definition.

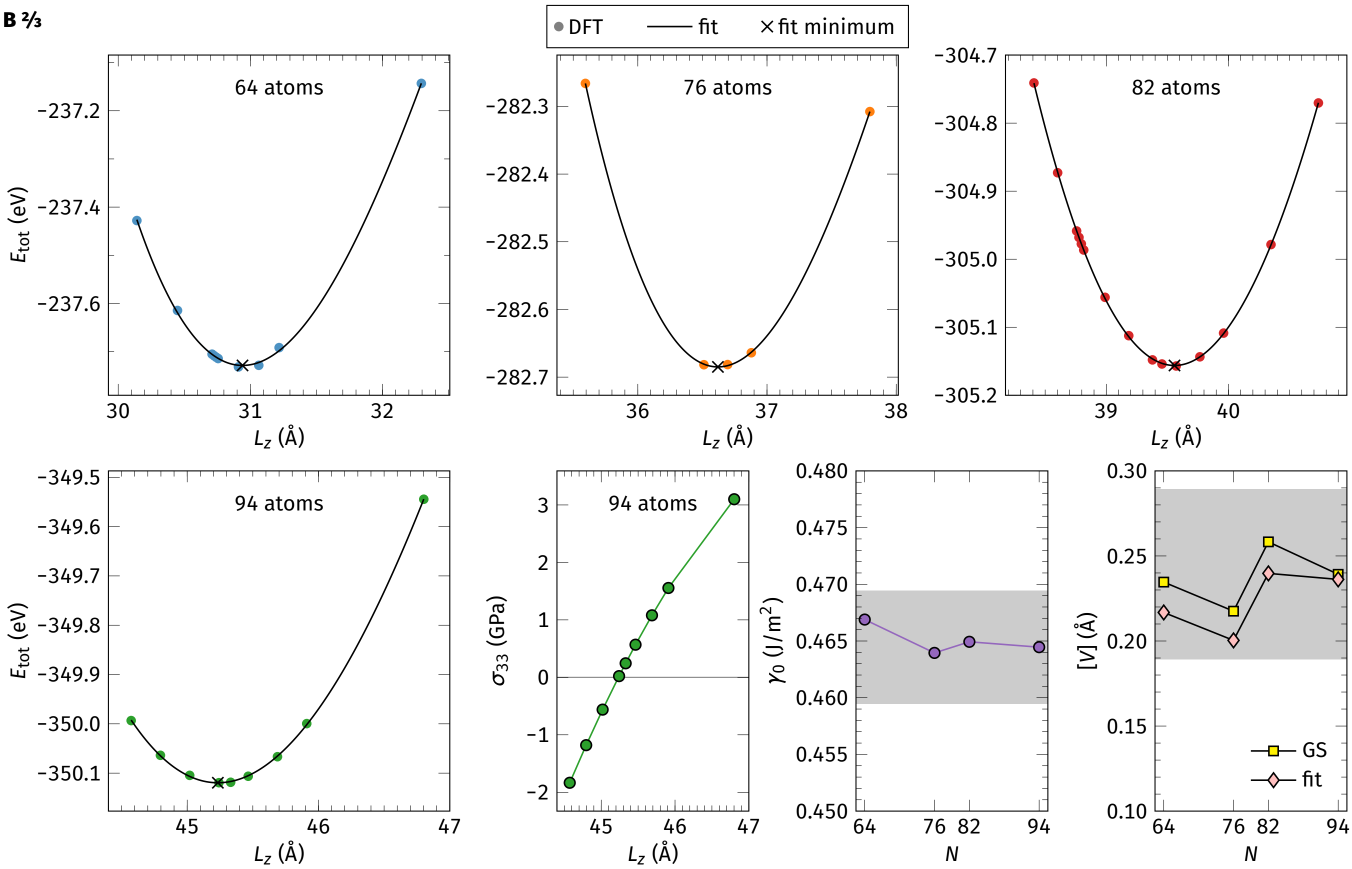


**Supplemental Fig. S8:** Same as Fig. S7, but for the "B ⅔" GB phase.

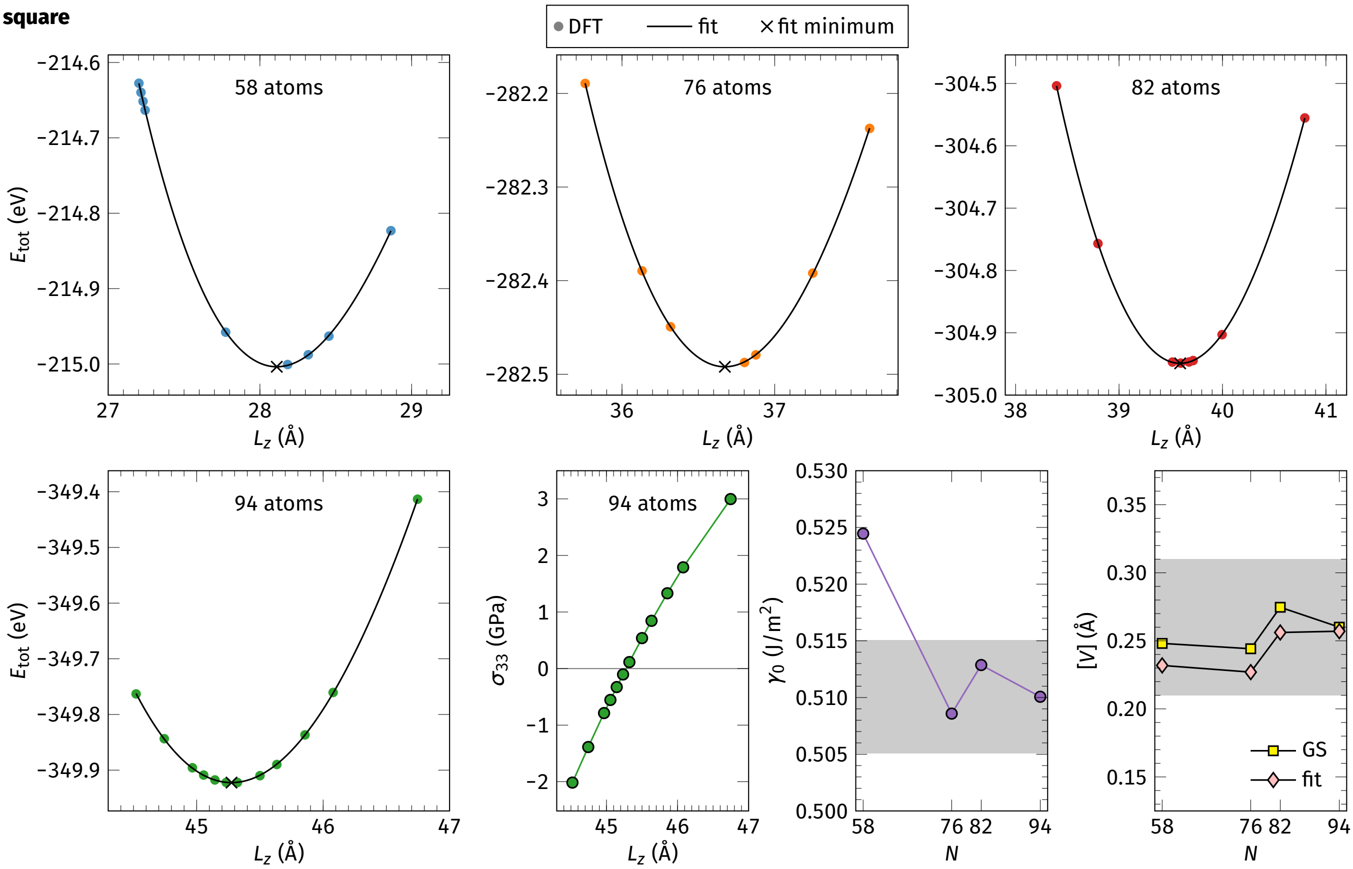


**Supplemental Fig. S9:** Same as Fig. S7, but for the "square" GB phase.

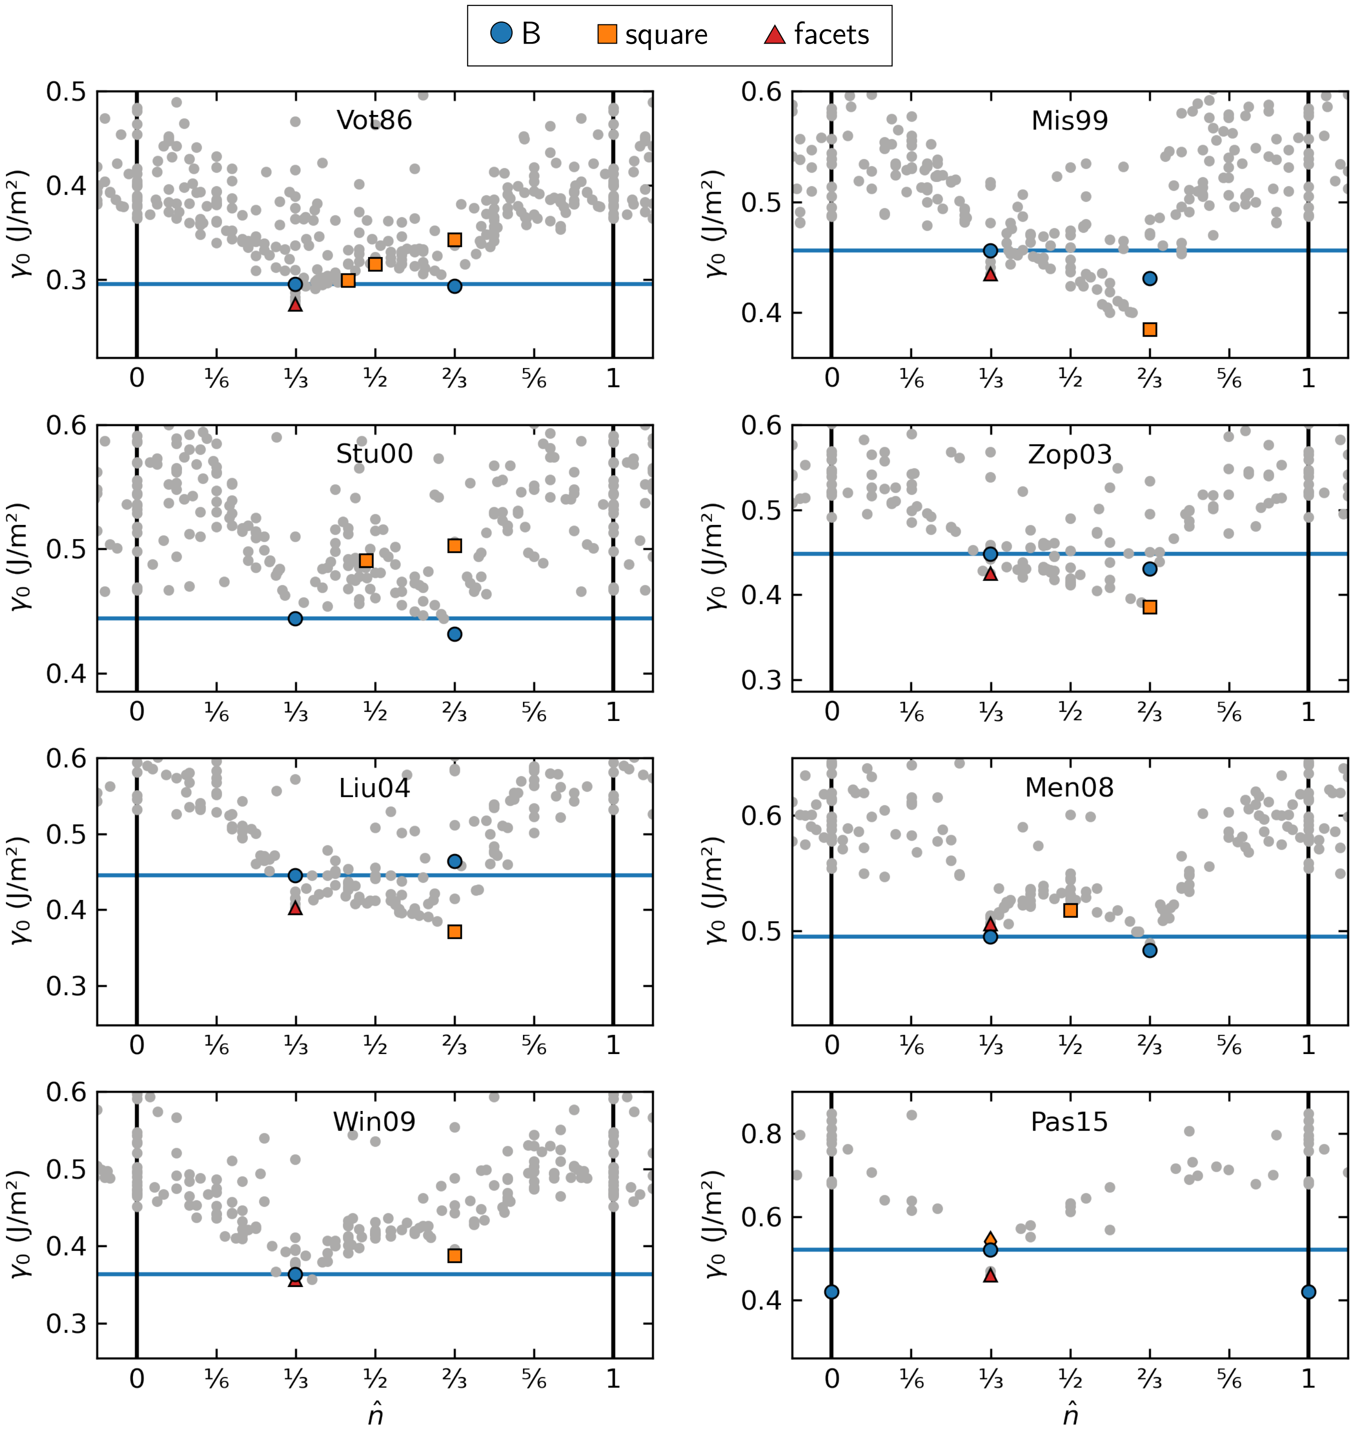


**Supplemental Fig. S10:** Structure search with GRIP for Σ3 $[11\bar{1}]$ (011) GBs with different potentials. The larger data points mark low-energy structures for the different GB phases. The horizontal blue line corresponds to the energy of the B ⅓ structure. According to our DFT calculations, it should be approximately equal to the energy of B ⅔ and significantly lower than the energy of the square phase. We can see that this is only true for the Vot86, Stu00, and Men08 potentials. The low-energy structures found in this structure search do not always correspond to the structures found with Zha09 and evaluated with DFT: Men08 is missing the ideal "square" structure at $\hat{n} = 2/3$, although this is possibly because its energy is so high that GRIP discards it. Win09 has no mechanically stable B ⅔ structure and Pas15 exhibits a low-energy B-like structure at $\hat{n} = 0$, but is missing the expected $\hat{n} = 2/3$ structures. These results agree with our conclusions from the appendix of the main paper.

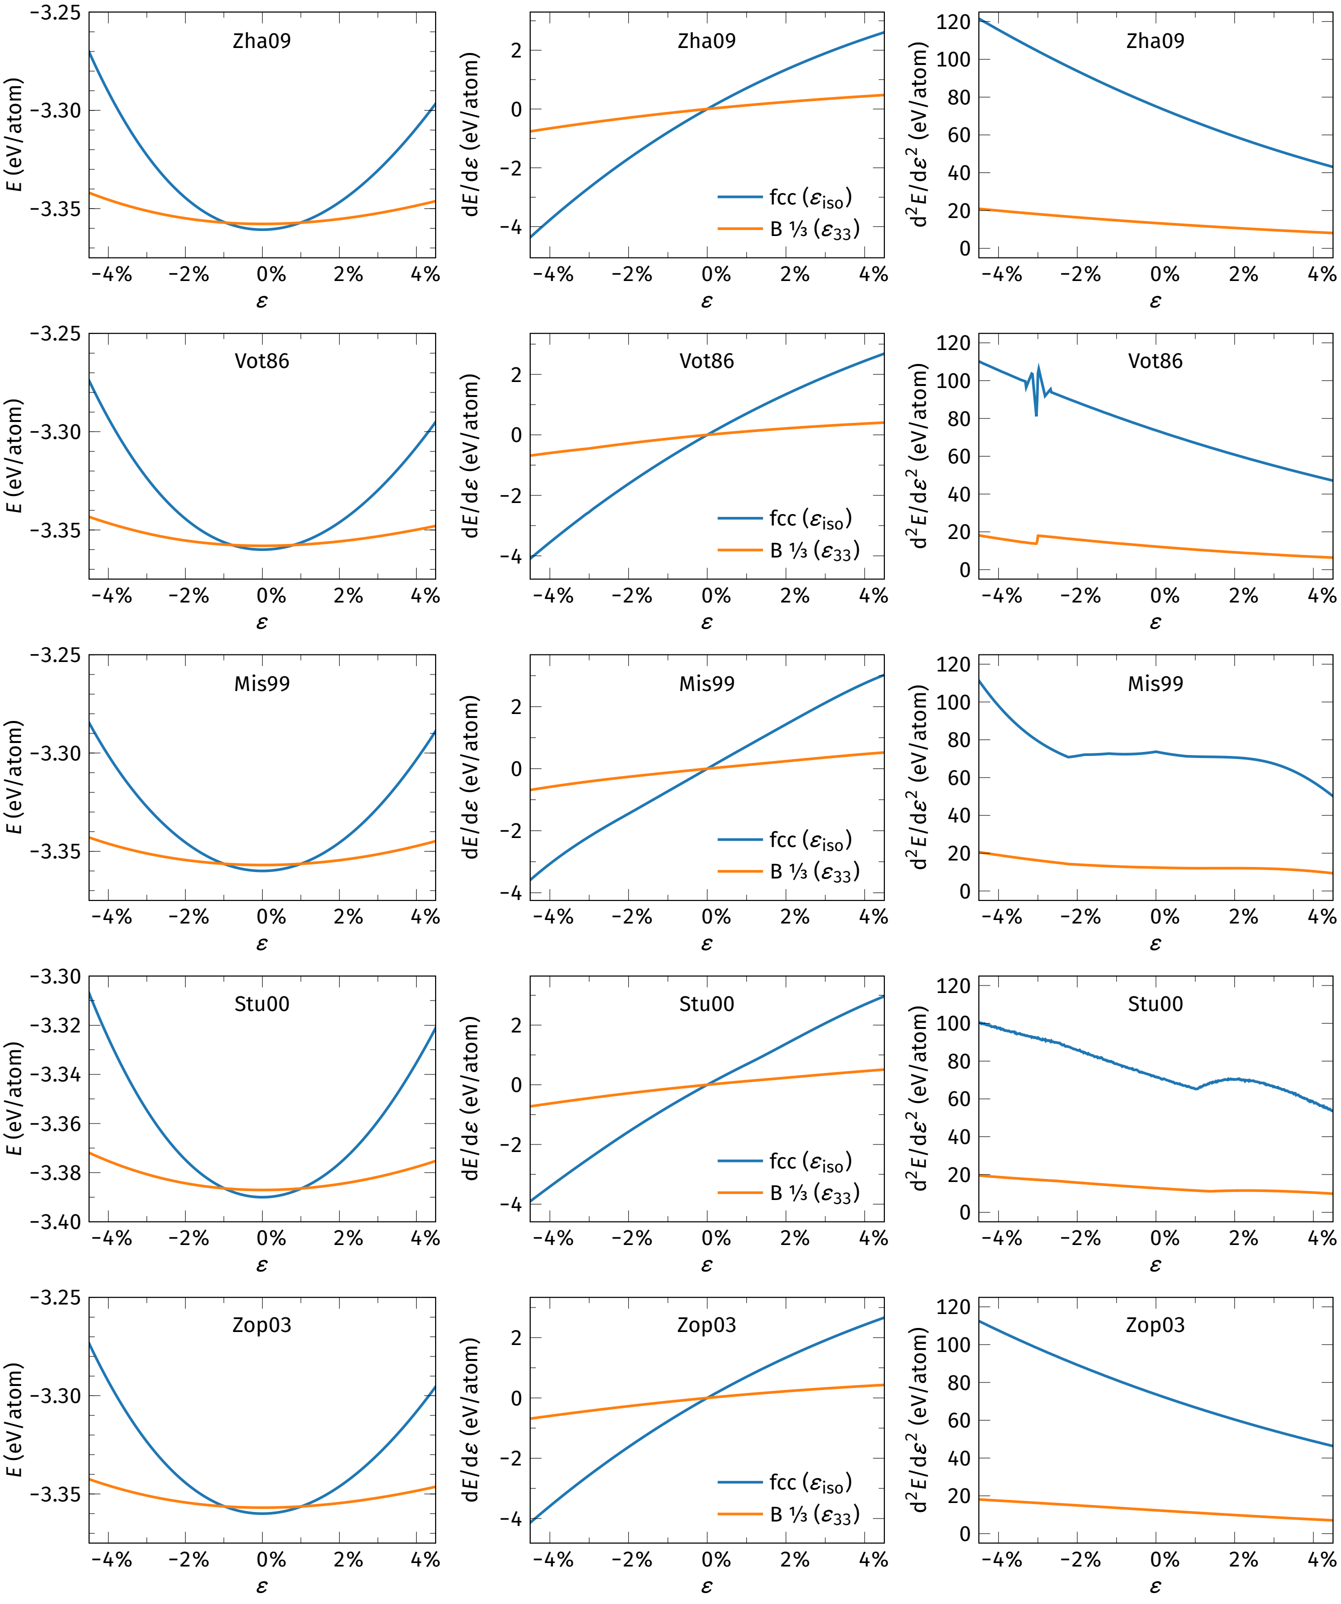


**Supplemental Fig. S11:** Energy and its first two derivatives of simulation cells with defect-free fcc, as well as with a B ⅓ GB, as a function of strain. The fcc cell was strained hydrostatically, while the GB cell was strained normal to the GB. The step size for the strain was 0.002% and the derivatives were obtained with the finite-difference method. No additional relaxation was performed. This data highlights numerical issues with the potentials: Noise in the second derivative is an amplification of noise existing in the original potential file and leads to noise in the force constant matrix. Non-continuous derivatives point towards unphysical shapes of the potential-energy function. Noise localized around one strain value points to numerical issues with the cutoff function, since likely a single atom enters or leaves the cutoff radius at that point. Here, Zha09 and Zop03 seem free of these issues. Continued in Supplemental Fig. S12.

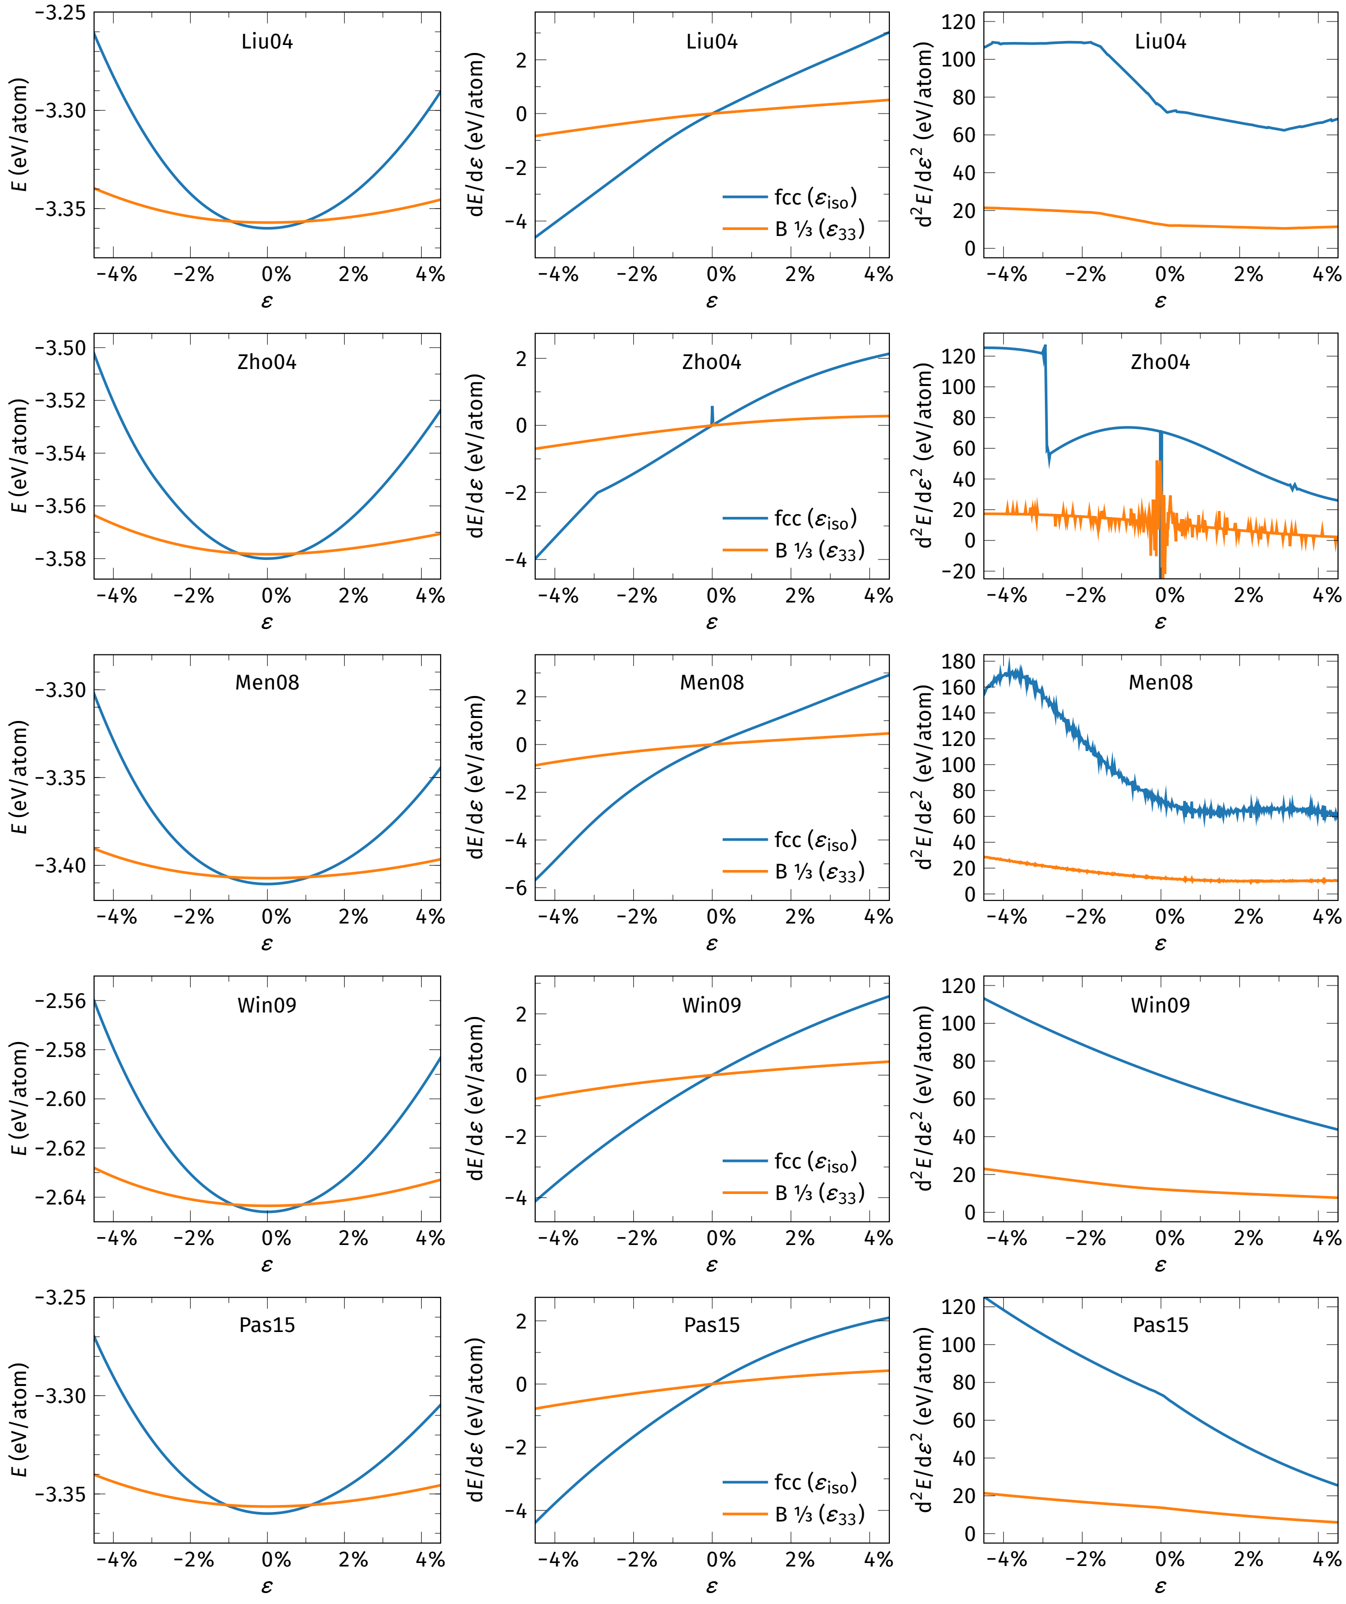


**Supplemental Fig. S12:** Continued from Supplemental Fig. S11. Only Win09 has smooth functions. Note in particular that Zho04 exhibits severe issues even at zero strain. This can explain why we were unable to get consistent values for the stacking-fault energy. Even small structural changes lead to fluctuations of the potential energy computed with Zho04. Men08, while otherwise performing quite well, has unphysical changes of curvature and some noise.
